# Supplementary material for: Supervised and Extended Restart in Random Walks for Ranking and Link Prediction in Networks
Source: arXiv:1710.06609 source file (2017-10-18)
Supplement: Supplementary file 1 [file 090appendix.tex]

\hide{

The equation of \model is as follows:
\begin{equation}
\label{eq:rwer}
\rr=\nA^\top  (\mat{I} - diag(\cc) ) \rr + \left(\cc^\top \rr \right) \qq
\end{equation}
where $\nA$ is a row-normalized matrix, $\cc$ is a restart vector whose $i$-th entry is $c_i$, $diag(\cc)$ is a matrix whose $diag(\cc)_{ii} = c_i$ and other entries are $0$, and $\qq$ is a vector whose $s$-th element is $1$, and all other elements are $0$.

%As in the case of RWR, \rwer can be expressed in the closed form.
%Since our method
The following lemma shows that equation~\eqref{eq:rwer} can be represented as a closed form equation.
\begin{lemma}
	%    [closed form solution of \rwer]
	\label{lemma:closed}
	The closed form w.r.t. $\rr$ in equation~\eqref{eq:rwer} is represented as follows:
	\begin{equation}
		\rr = (\mat{I} - \mat{B})^{-1} \qq
	\end{equation}
	where $\mat{B}$ is $\nA^\top (\mat{I} - diag(\cc) ) + \left(\qq (\cc - \mat{1})^\top \right)$, $\nA$ is a row-normalized matrix% (i.e., $\nA=\mati{D}\mat{A}$ and $\mat{D}$ is an out-degree diagonal matrix)
, and $\vect{1}$ is an all-ones vector.

\begin{proof}
	Note that $\vectT{c}\vect{r}$ is a scalar; thus, $(\vectT{c}\vect{r})\vect{q} = \vect{q}(\vectT{c}\vect{r}) = (\vect{q}\vectT{c})\vect{r}$.
	Hence, equation~\eqref{eq:rwer} is represented as follows:
	\begin{align*}
	\rr & = \nA^\top (\mat{I} - diag(\cc)) \rr + \left(\qq \cc^\top \right) \rr\\
	&= \nA^\top (\mat{I} - diag(\cc)) \rr + \left(\qq \cc^\top \right) \rr - \vect{q} + \vect{q}
	\end{align*}
	Since $\vect{r}$ is a probability vector and $\vectT{1}\vect{r}=1$, the above equation is written in the following equation:
	\begin{align*}
	\rr &=     \nA^\top (\mat{I} - diag(\cc)) \rr + \left(\qq \cc^\top \right) \rr - \vect{q}\left(\vectT{1}\vect{r}\right) + \vect{q} \\
	& = \nA^\top (\mat{I} - diag(\cc) ) \rr + \left(\qq (\cc - \mat{1})^\top \right) \rr + \qq\\
	& = \left(\nA^\top (\mat{I} - diag(\cc) ) + \qq (\cc - \mat{1})^\top \right)\rr + \qq\\
	& = \mat{B} \rr + \qq
	\end{align*}
	where $\mat{B}$ is $\nA^\top (\mat{I} - diag(\cc) ) + \qq (\cc - \mat{1})^\top$.
	Finally, $\vect{r}$ is represented in the following closed form:
	\begin{equation*}
	\rr = (\mat{I} - \mat{B})^{-1} \qq
	\end{equation*}
	Note that $\mat{I} - \mat{B}$ is invertible (see the following Lemma~\ref{lemma:invertible}).
	%In order to get the closed form of Equation~\ref{eq:rwer}, a constant term is needed.
	%    \begin{equation*}
	%    \label{eq:closed}
	%    \begin{split}
	%    \rr & = \nA^\top  \left( \mat{I} - diag(\cc) \right) \rr + \left(\cc^\top \rr \right) \qq \\
	%    & = \nA^\top (\mat{I} - diag(\cc)) \rr + \left(\qq \cc^\top \right) \rr\\
	%    & = \nA^\top (\mat{I} - diag(\cc) ) \rr + \left(\qq (\cc - \mat{1})^\top \right) \rr + \qq\\
	%    & = \left(\nA^\top (\mat{I} - diag(\cc) ) + \qq (\cc - \mat{1})^\top \right)\rr + \qq\\
	%    & = \mat{B} \rr + \qq
	%    \end{split}
	%    \end{equation*}
	%    where $\mat{B}$ is $\nA^\top (\mat{I} - diag(\cc) ) + \qq (\cc - \mat{1})^\top$. $\left(\cc^\top \rr \right) \qq$ in Equation~\ref{eq:rwer} becomes $\left(\qq \cc^\top \right) \rr$ in the second equality by using commutative and associative properties.
	%    Therefore, $\rr = (\mat{I} - \mat{B})^{-1} \qq$.
\end{proof}
\end{lemma}

}

\begin{lemma}
	\label{lemma:invertible}
	Let $\mat{B} = \nA^\top (\mat{I} - diag(\cc) ) + \qq (\cc - \mat{1})^\top$. Then, $\mat{M} = \mat{I} - \mat{B}$ is invertible.
	\begin{proof}
		Let $\mat{C}$ be $\mat{I} - diag(\cc)$, and $\mat{X}$ be $\mat{I} -\nA^\top\mat{C}$. Then, $\mat{M} = \mat{I} - \mat{B}$ is represented as follows:
		\begin{align*}
			\mat{M} &= \mat{I} -\nA^\top\mat{C} - \qq (\cc - \mat{1})^\top \\
			&= \mat{X} + \qq(\mat{1} - \cc)^\top
		\end{align*}
		Note that $(\nA^\top\mat{C})_{ij} \geq 0$, $1 \leq i, j \leq n$ and the largest eigenvalue $\lambda_{max}(\nA^\top\mat{C}) \leq 1$ since $\nA$ is stochastic and $\mat{C}$ is sub-stochastic.
		In other words, $\mat{X}=\mat{I} - \nA^\top\mat{C}$ is an M-matrix~\cite{fujimoto2004two}; thus, $\mati{X}$ exists and all entries of $\mati{X}$ are nonnegative.
%		$\mati{X} \succeq 0$ (i.e., $\mat{X}$ is inverse-positive).
		By Sherman-Morrison lemma~\cite{sherman1950adjustment}, $(\mat{X} + \qq (\mat{1} - \cc)^\top)^{-1}$ is represented as follows:
		\begin{equation*}
			\left(\mat{X} + \qq(\mat{1} - \cc)^\top\right)^{-1} = \mati{X} - \frac{\mati{X}\vect{q}(\vect{1}-\vect{c})^{\top}\mati{X}}{1 + (\vect{1}-\vect{c})^{\top}\mati{X}\vect{q}}
		\end{equation*}
		Since all entries of $\mati{X}$, $\vect{1}-\vect{c}$ and $\vect{q}$ are nonnegative,  $(\vect{1}-\vect{c})^{\top}\mati{X}\vect{q} \geq 0$; thus, $ 1 + (\vect{1}-\vect{c})^{\top}\mati{X}\vect{q} \geq 1$.
Since the inverse of $\mat{X} + \qq(\mat{1} - \cc)^\top$ exists iff $X$ is invertible and $ 1 + (\vect{1}-\vect{c})^{\top}\mati{X}\vect{q} \neq 0$, $\mat{I} - \mat{B}$ is invertible.
%
%		Hence, the right side of the above equation exists, i.e., $\left(\mat{X} + \qq(\mat{1} - \cc)^\top\right)^{-1}=\mati{M}$ exists.
%		$\mat{I} - \mat{B}^{\top}$ is also invertible, which is proved similarly to the proof of $\mat{I} - \mat{B}$.
		%\QEDA
	\end{proof}
\end{lemma}

\hide{

\newpage
\begin{figure}[t!]
	\centering
	%	\vspace{2mm}
	%	\centerline{\includegraphics[width=0.4\linewidth]{FIG/restart/label4.PNG}}
	\hspace{-5mm}
	%	\vspace{3mm}
	\subfigure[MAP in the Polblogs dataset. Positive nodes are randomly chosen.]
	{
%		\label{fig:exp:restart:map:hepph}
		\includegraphics[width=0.7\linewidth]{FIG/restart/POL_MAP_random}
	}

	\caption{
%		\label{fig:exp:restart}
		%		Parameter sensitivity of our method \sure and RWR in the Polblogs and Cora dataset.
		%		We report the link prediction accuracy using MAP measure,
		%		changing the values of the elements in the origin vector $\vect{o}$ in \sure, and the restart probability $c$ of RWR.
		%		Note that \sure is less sensitive to varying values of the parameter than RWR is, since \sure learns the optimal random walk from data.
		%		Furthermore, \sure always outperforms RWR regardless of the parameter settings.
		\blue{Parameter sensitivity of our method \sure in the Polblogs and Cora dataset.
			We report the ranking and link prediction accuracy using MAP measure,
			changing the values of the elements in the origin vector $\vect{o}$ in \sure.
			Note that \sure is less sensitive to varying values of the parameter than RWR is, since \sure learns the optimal random walk from data.
			Furthermore, \sure always outperforms RWR regardless of the parameter settings.}
	}
\end{figure}

}

%\begin{lemma}
%	\label{lemma:method:Mx}
%	%    \vspace{-3mm}
%	Suppose that $\MM(x,:)^\top$ is $\tilde{\rr}$.
%	Then, $\tilde{\rr}$ is computed iteratively until convergence $(\lVert\tilde{\rr}^{(t+1)} - \tilde{\rr}^{(t)}\rVert < \epsilon)$ by the following update rule:
%	\begin{equation*}
%		%        \vspace{-1mm}
%		\tilde{\rr}^{(t+1)} \leftarrow (\mat{I} - diag(\cc) ) \nA \tilde{\rr}^{(t)} + (\cc - \mat{1}) \qq^\top \tilde{\rr}^{(t)} + \mat{p}
%	\end{equation*}
%	where $\mat{p}$ is an $n \times 1$ vector whose $x$-th element is $1$, and the others are $0$.
%	%\red{Note that $\tilde{\rr}^{(t)}$ converges to $(\mat{I}-\mat{B}^\top)^{-1} \mat{p} = \MM(x,:)^\top$ as $t\rightarrow \infty$.}
%	\begin{proof}
%		$\MM(x,:)^\top$ is a column vector which is the transpose of the $x$-th row of the matrix $\MM$.
%		In other words, $\MM(x,:)^\top = \MM^\top \mat{p}$.
%		Let $\MM(x,:)^\top$ be $\tilde{\rr}$.
%		Then, $\tilde{\rr}$ is represented as follows:
%		\begin{equation*}
%			\tilde{\rr} = \MM^\top \mat{p}= (\mat{I}-\mat{B}^\top)^{-1} \mat{p} \Leftrightarrow  \tilde{\rr} = \mat{B}^\top \tilde{\rr} + \mat{p}
%		\end{equation*}
%		where $\mat{B} = \nA^\top (\mat{I} - diag(\cc) ) + \qq (\cc - \mat{1})^\top $.
%	\end{proof}
%\end{lemma}
